# Supplementary material for: INVE: Interactive Neural Video Editing
Source: arXiv:2307.07663 source file (2023-07-15)
Supplement: Supplementary file 1 [file 6_appendix.tex]

\appendix
\section{Switching Times}

In this appendix...
